# Supplementary material for: Rebalance and Smear for Multi-jet Background Estimation
Source: arXiv:2206.09583 source file (2022-07-30)
Supplement: Supplementary file 1 [file appendix_simulation.tex]

\section{More simulation details}
\label{app:simulation}

In total, 2650000 for QCD, 30750000 for $W$ and $Z$ boson processes, 2000000 for $\t\bar{t}$, and 600000 signal events have been produced.
